# Supplementary material for: Watch Your Step: Learning Node Embeddings via Graph Attention
Source: arXiv:1710.09599 source file (2018-09-12)
Supplement: Supplementary file 1 [file nips_appendix.pdf]

## 7 Appendix

### 7.1 Step-by-step Derivation of Equation (6)

Let  $x(k)$  be the position of random surfer at time  $k$ . Specifically,  $x : \mathbb{Z}^+ \rightarrow V$ . We assume a Markov chain: The value of  $x(k)$  only depends on previous step:  $x(k-1)$ . To calculate the expectation  $\mathbb{E}[\mathbf{D}]$ , the square node-to-node co-occurrence matrix, we start by calculating one entry at a time:  $\mathbb{E}[D_{uv}]$ , the expected number of times that  $u$  is selected in  $v$ 's context. Let  $W_v(k)$  be the context that gets sampled if  $v$  is visited at the  $k^{\text{th}}$  step. Concretely, if  $x(k) = v$ , and the random walker continues the sequence,  $x(k+1) = v'_1 \rightarrow x(k+2) = v'_2 \rightarrow x(k+3) = v'_3 \dots$ , then the context set of DeepWalk can be defined as  $W_v(k) = \{v_j \mid j \geq c\}$ , where  $c \sim \mathcal{U}\{1, C\}$ . We would like to count the event  $u \in W_v(k)$  for every  $k \in \{1, 2, \dots, C\}$ .

Using Markov Chain, we can write:

$$\begin{aligned} \Pr(x(i+k) = u \mid x(i) = v) &= \Pr(x(k) = u \mid x(0) = v) \\ &= (\mathcal{T}^k)_{uv} \end{aligned} \quad (11)$$

Now, if node  $u$  was visited  $k$  steps after node  $v$ , then the probability of it being sampled is given by:

$$\Pr(u \in W_v(k) \mid x(k) = u, x(0) = v). \quad (12)$$

In case of DeepWalk [30], probability above equals:

$$\Pr(k \leq c \mid x(k) = u, x(0) = v) \text{ where } c \sim \mathcal{U}\{1, C\}, \quad (13)$$

and event  $k \leq c$  is independant of the condition  $(x(k) = u \cap x(0) = v)$ . Further, event  $k \leq c$  can be partitioned and Eq. (13) can be written as

$$\Pr(c = k \cup c = k+1 \cup \dots \cup c = C) \quad (14)$$

$$= \sum_{j=k}^C \Pr(c = j) \quad (15)$$

$$= (C - k + 1) \left( \frac{1}{C} \right) = 1 - \frac{k-1}{C}, \quad (16)$$

where second line is trivial since the events  $c = j$  are disjoint. We can now use Bayes' rule to derive the probability of  $u$  being visited  $k$  steps after  $v$  and being selected in  $v$ 's sampled context, as:

$$\begin{aligned} \Pr(u \in W_v(k), x(k) = u \mid x(0) = v) \\ &= \Pr(u \in W_v(k) \mid x(k) = u, x(0) = v) \Pr(x(k) = u \mid x(0) = v) \\ &= \left( 1 - \frac{k-1}{C} \right) (\mathcal{T}^k)_{uv} \end{aligned} \quad (17)$$

Now, let  $E_{vku}$  be the event that a walker visits  $v$  and after  $k$  steps, visits  $u$  and selects it part of its context. This event happens with the probability indicated in Equation 17. Concretely,

$$\mathbb{E}[E_{vku} \mid x(0) = v] = \left( 1 - \frac{k-1}{C} \right) (\mathcal{T}^k)_{uv}. \quad (18)$$

Let  $E_{v*u}$  count the events  $\{E_{vku} : k \in [1, C]\}$ , then:

$$\mathbb{E}[E_{v*u} \mid x(0) = v] = \mathbb{E} \left[ \sum_{k=1}^C E_{vku} \mid x(0) = v \right] \quad (19)$$

$$= \sum_{k=1}^C \mathbb{E}[E_{vku} \mid x(0) = v] = \sum_{k=1}^C \left( 1 - \frac{k-1}{C} \right) (\mathcal{T}^k)_{uv}. \quad (20)$$

Suppose we run DeepWalk, starting  $m$  random walks from each node  $v$ , then the expected number of times that  $u$  is present in the context of  $v$  is given by:

$$\mathbb{E}[D_{uv}^{\text{DEEPWALK}}] = m \mathbb{E}[E_{v*u} \mid x(0) = v] = m \sum_{k=1}^C \left( 1 - \frac{k-1}{C} \right) (\mathcal{T}^k)_{uv}.$$

401 Finally, we can write down the expectation over the square matrix  $\mathbf{D}$ :

$$\begin{aligned}\mathbb{E} [\mathbf{D}^{\text{DEEPWALK}}] &= \text{diag}(m, m, \dots, m) \sum_{k=1}^C \left(1 - \frac{k-1}{C}\right) (\mathcal{T}^k) \\ &= \text{Equation (6)}\end{aligned}$$

402

□

### 403 7.1.1 Choice of $\tilde{\mathbf{P}}^{(0)}$

404 Random walk simulation of node2vec [13] starts 80 walks from every graph node  $v \in V$ . Therefore,  
 405 in our experiments, we set  $\tilde{\mathbf{P}}^{(0)} := \text{diag}(80, 80, \dots, 80)$ . This initial condition yields  $D_{vu}$  to be  
 406 the expected number of times that  $u$  is visited if we started 80 walks from  $v$ . There can be other  
 407 reasonable choices. Nonetheless, we use what worked well in practice for [14, 30]. We leave the  
 408 search for a better  $\tilde{\mathbf{P}}^{(0)}$  as future work.
